# Supplementary material for: Molecular structure, binding, and disorder in TDBC-Ag plexcitonic assemblies
Source: arXiv:2601.22022 ancillary file (2026-01-29)
Supplement: Supplementary file 1 [file Supporting_Information.pdf]

# Supporting Information: Molecular structure, binding, and disorder in TDBC–Ag plexcitonic assemblies

J. Baños-Gutiérrez,[1] R. Bercy,[2] Y. García Jomaso,[3] S. Balci,[4] G. Pirruccio,[3] J. Halldin Stenlid,[5] M.J. Llansola-Portoles,[2] and D. Finkelstein-Shapiro[1,*]

[1] *Instituto de Quimica, Universidad Nacional Autonoma de Mexico, Circuito Exterior, Ciudad Universitaria, Alcaldía Coyoacán C.P. 04510, Ciudad de Mexico*
[2] *CEA, CNRS, Institute for Integrative Biology of the Cell (I2BC), Université Paris-Saclay, 91190 Gif-sur-Yvette, France*
[3] *Instituto de Física, Universidad Nacional Autónoma de México, Apartado Postal 20-364, Ciudad de México, C.P. 01000, Mexico.*
[4] *Department of Photonics, Izmir Institute of Technology, 35430 Izmir, Turkey*
[5] *Department of Chemistry and Chemical Engineering, Chalmers University of Technology, Kemivägen 10, SE-412 96, Gothenburg, Sweden*

## CONTENTS

I. Solvent-dependent aggregation 2

II. NMR of purified TDBC 4
A. NMR of as-received TDBC 8

III. Raman scattering measurements 16

IV. Vibrational mode assignment 17

References 18

* daniel.finkelstein@iquimica.unam.mx

## I. SOLVENT-DEPENDENT AGGREGATION

We can control the species present in solution (monomer or aggregate) by varying the fraction of MeOH and $H_2O$, and determine the relative composition via their optical absorption. Fig. S1 shows the optical absorption of TDBC in several MeOH and $H_2O$ mixtures at a concentration of 0.5 mg/mL. We can appreciate the gradual transition from monomer to aggregate.

This transition can be monitored by $^1$H NMR spectra as well (Fig. S2), for TDBC as received from Few Chemicals. At higher concentrations, the aggregate form is preferred even in higher ratios of MeOH:$H_2O$.

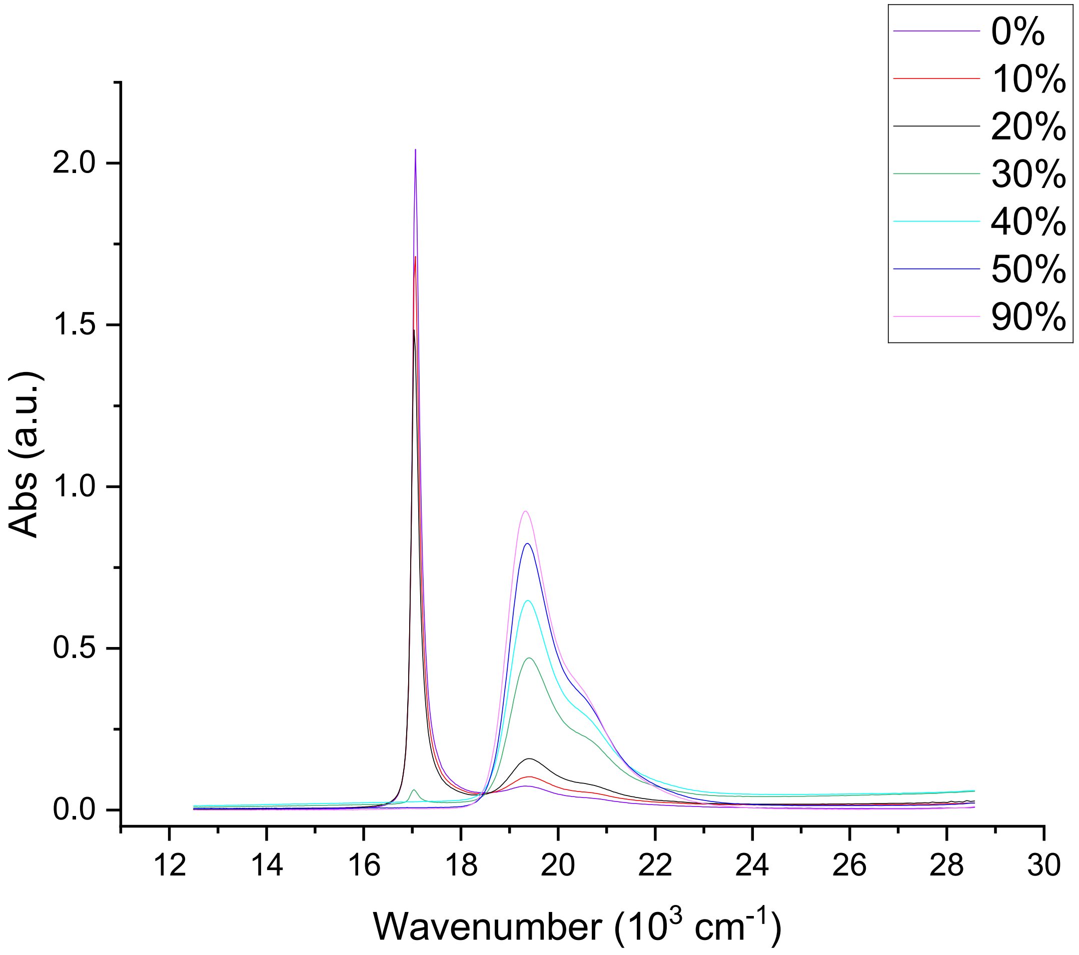


FIG. S1. TDBC absorption spectra by changing the percentage of methanol in the sample.

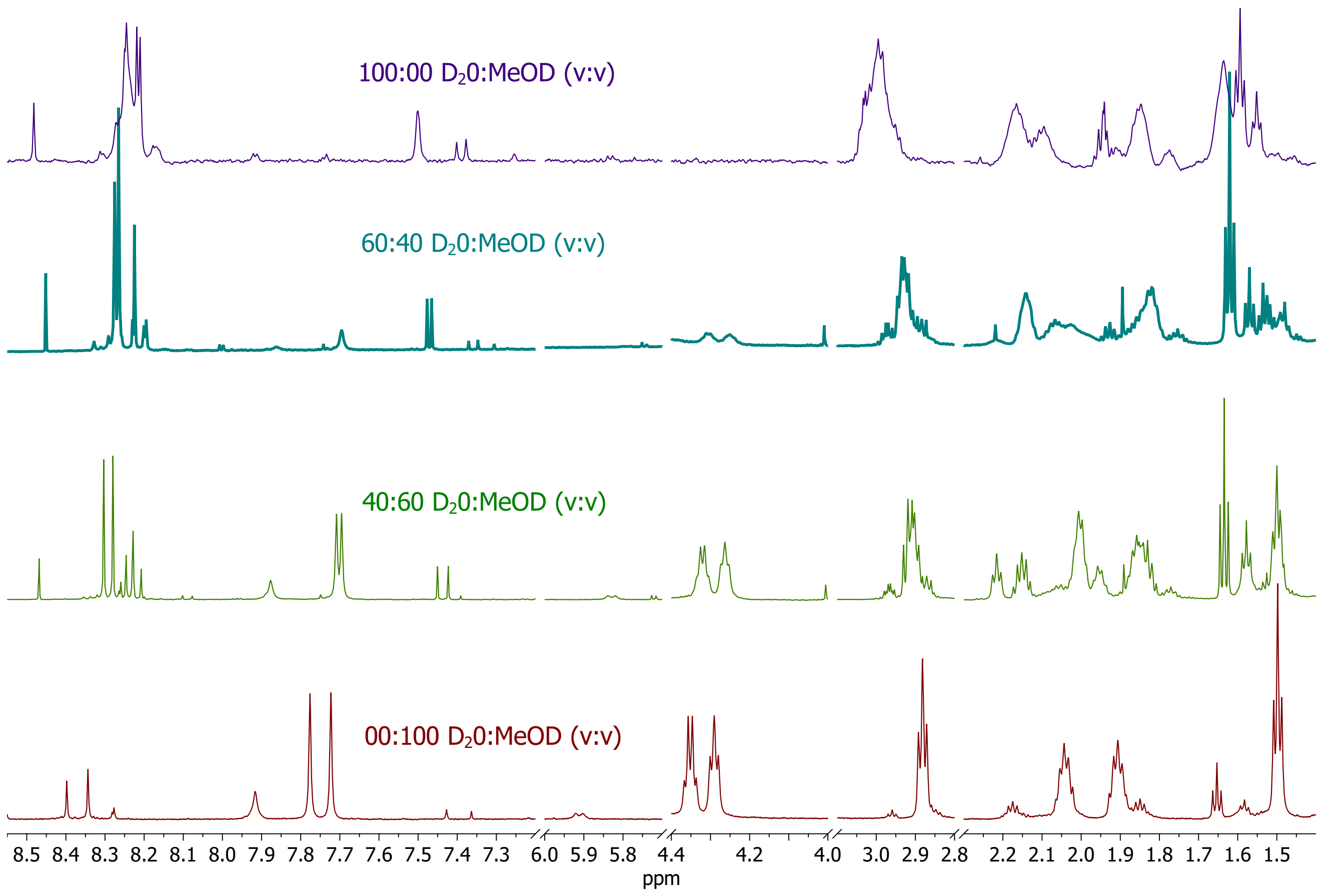


FIG. S2. $^1$H NMR spectra with increasing MeOH:$H_2O$ fractions.

## II. NMR OF PURIFIED TDBC

We provide the 1D $^1$NMR assingment of TDBC in different environments following the purification detailed in the main text. Fig. S2 shows the assignments in methanol while S3 shows the assignments in 6:4 MeOH:$H_2O$. We note that we only observe a single resonance per proton and UVvis at these concentrations confirms that they contain mostly monomer and aggregate, respectively. We also note that the integration of protons 12 and 14 according to the diagram of Figs. S2-S3 ($H_2$ and $H_2^*$ in the nomenclature of the main text) is very sensitive to the degree of aggregation as well as purity of the sample (see below).

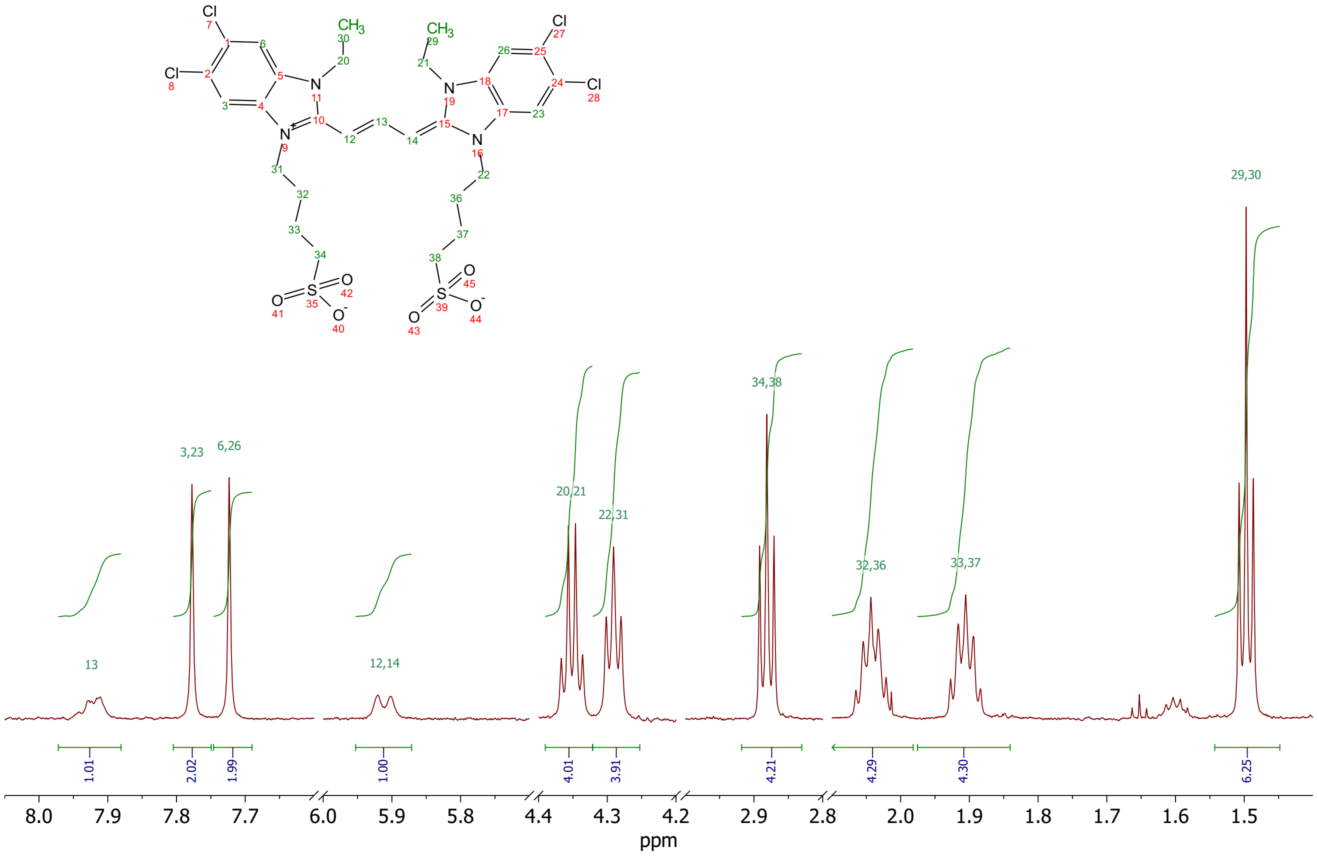


FIG. S3. $^1$H NMR of purified TDBC in 100% MeOH

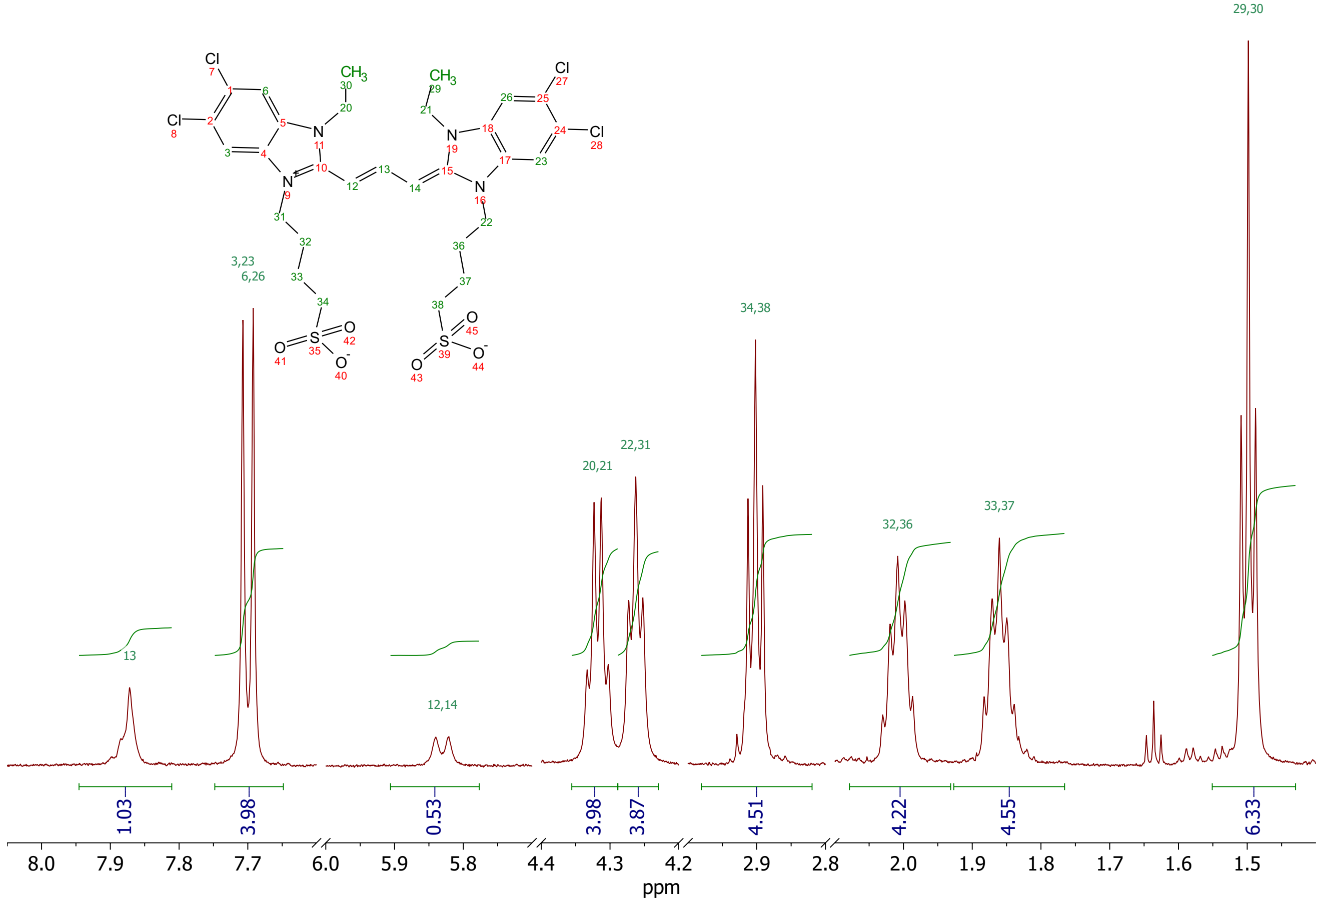


FIG. S4. $^1$H NMR of purified TDBC in 60% MeOH

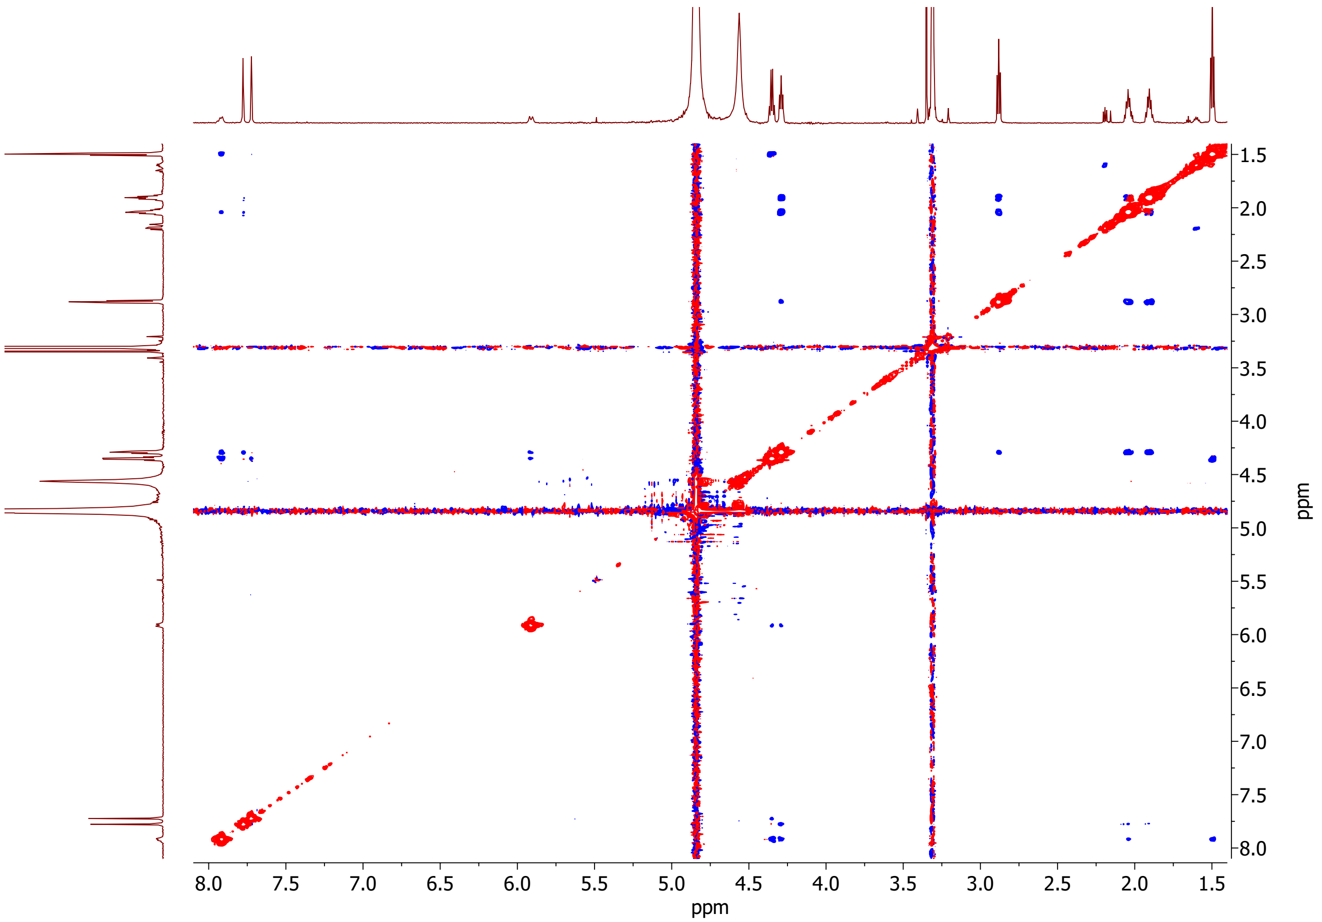


FIG. S5. NOESY spectrum of TDBC in methanol. Red contours correspond to negative phase, while blue contours correspond to positive phase.

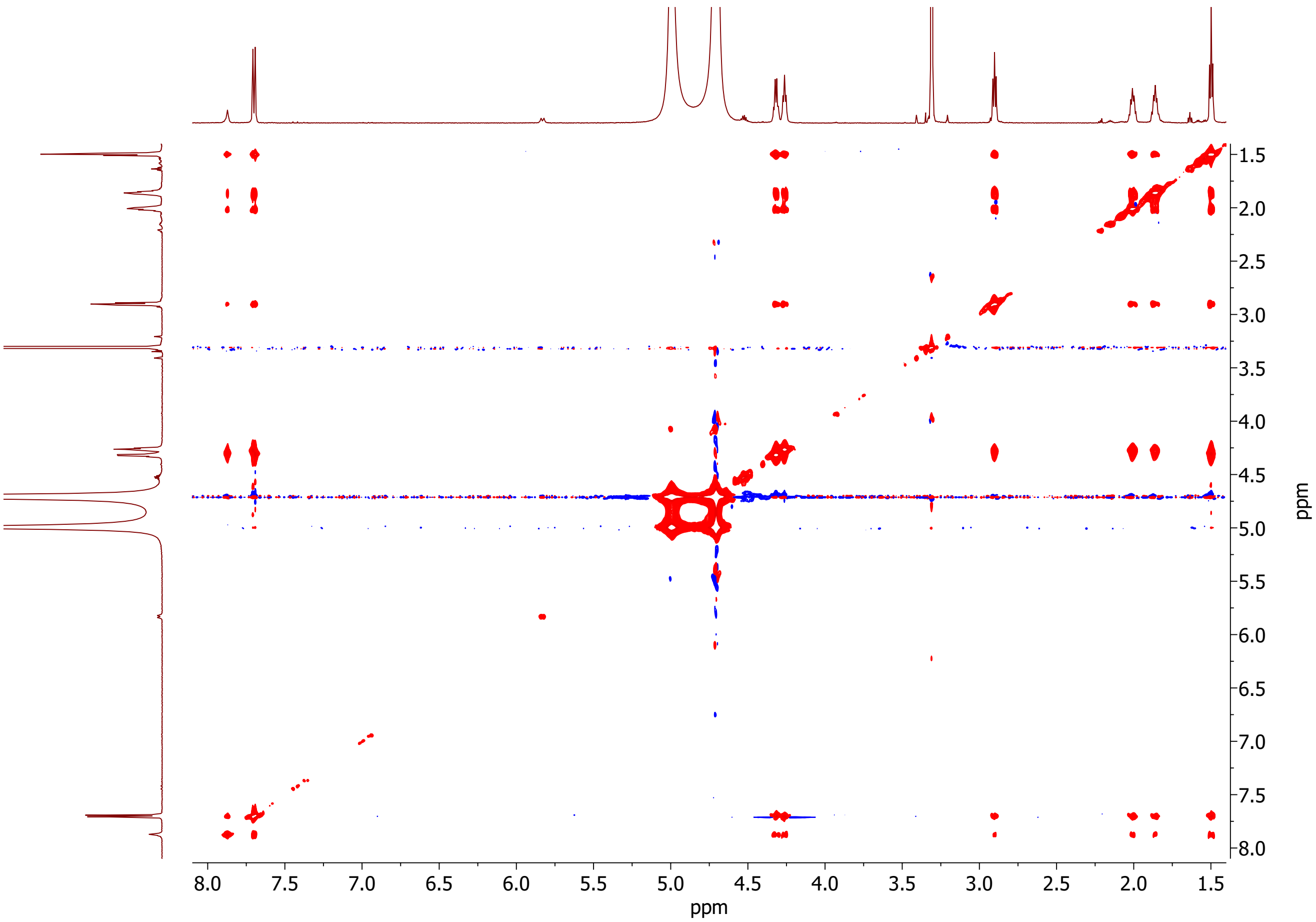


FIG. S6. NOESY spectrum of TDBC in 6:4 (v/v) MeOH:$H_2O$ mixture. Red contours correspond to negative phase, while blue contours correspond to positive phase.

### A. NMR of as-received TDBC

TDBC degrades under ambient conditions, resulting in the presence of impurities which affect the NMR spectra. We provide those spectra for reference in Figs. S7-15. Fig. S12 shows the $^1$H spectrum of concentrated plexcitons.

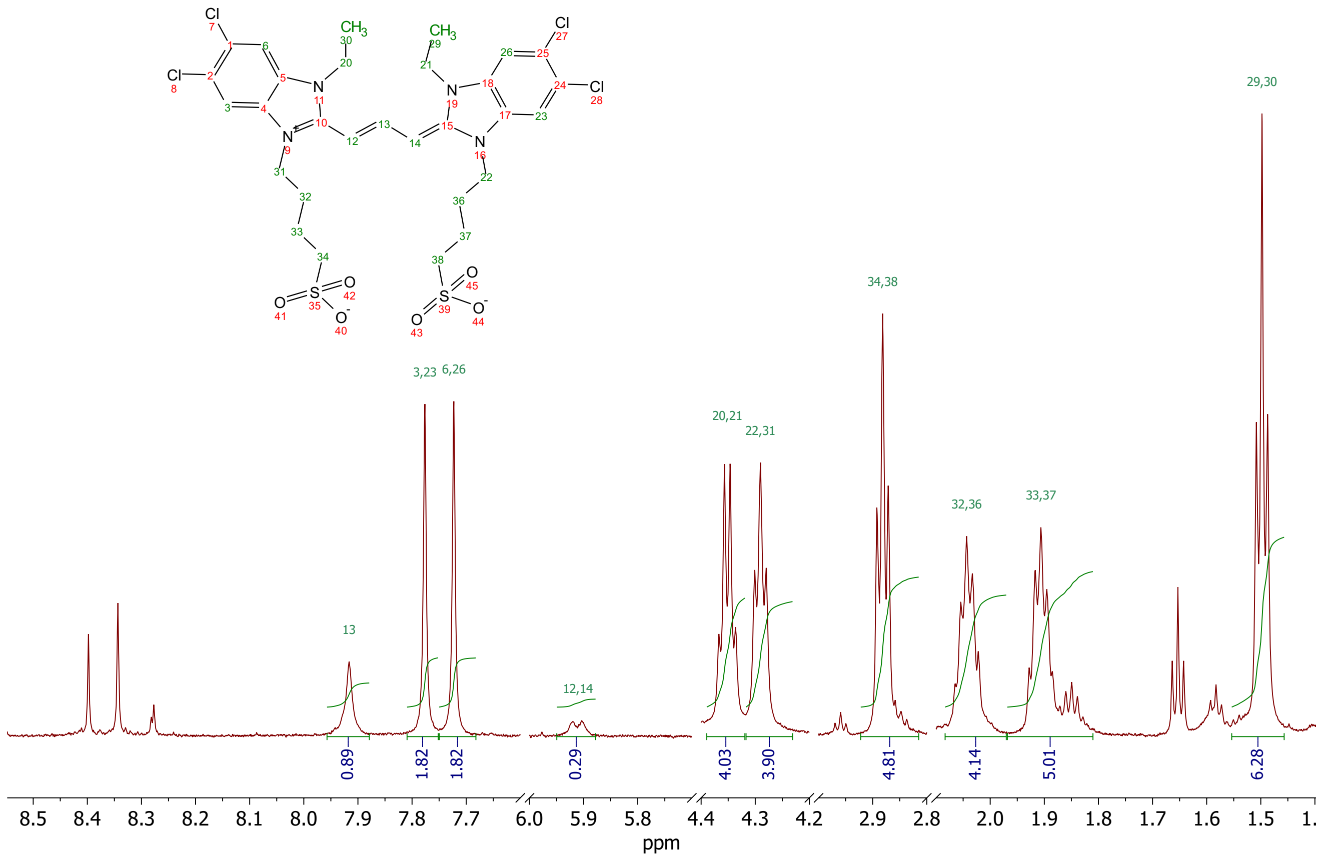


FIG. S7. $^1H$ NMR of TDBC in 100% MeOH

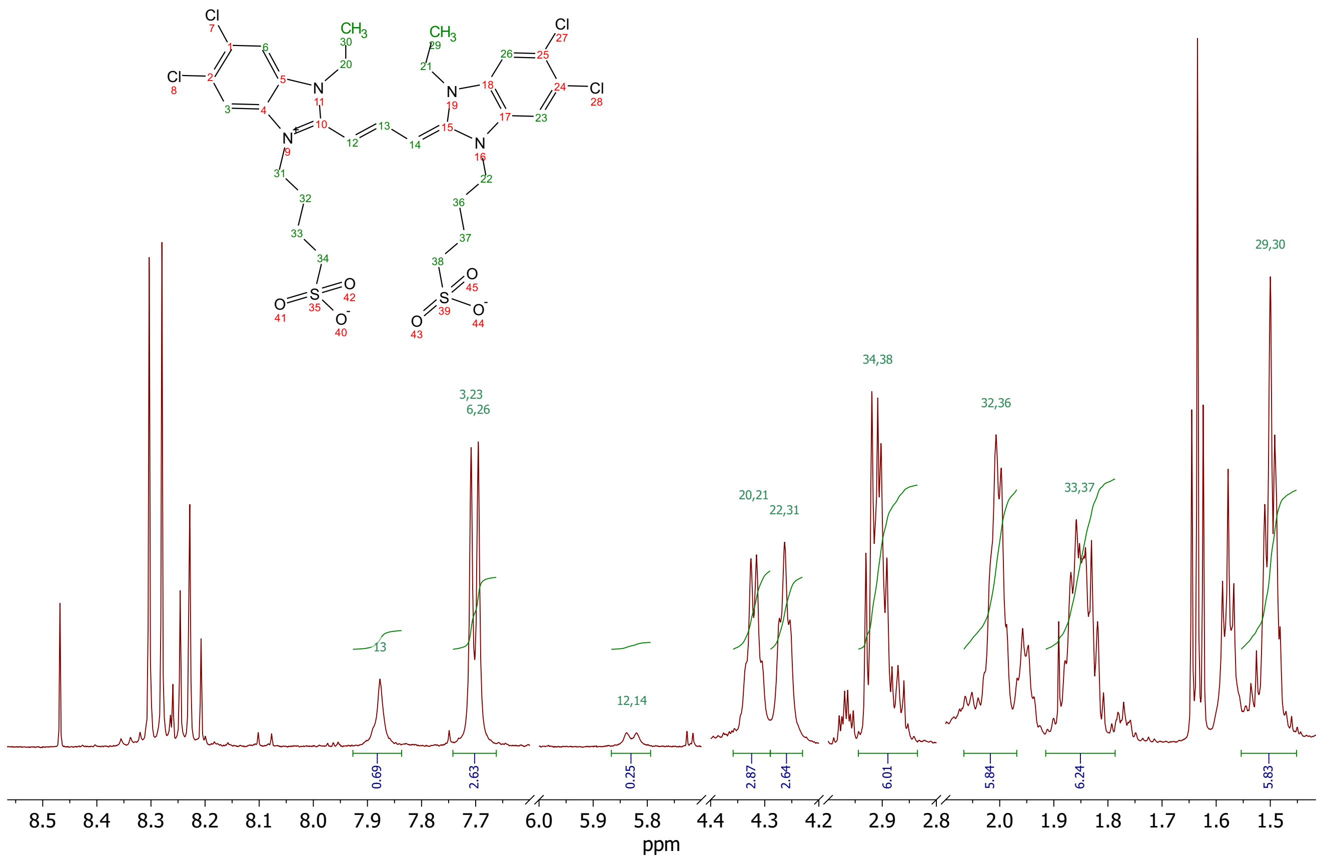


FIG. S8. $^{1}H$ NMR of TDBC in 60% MeOH

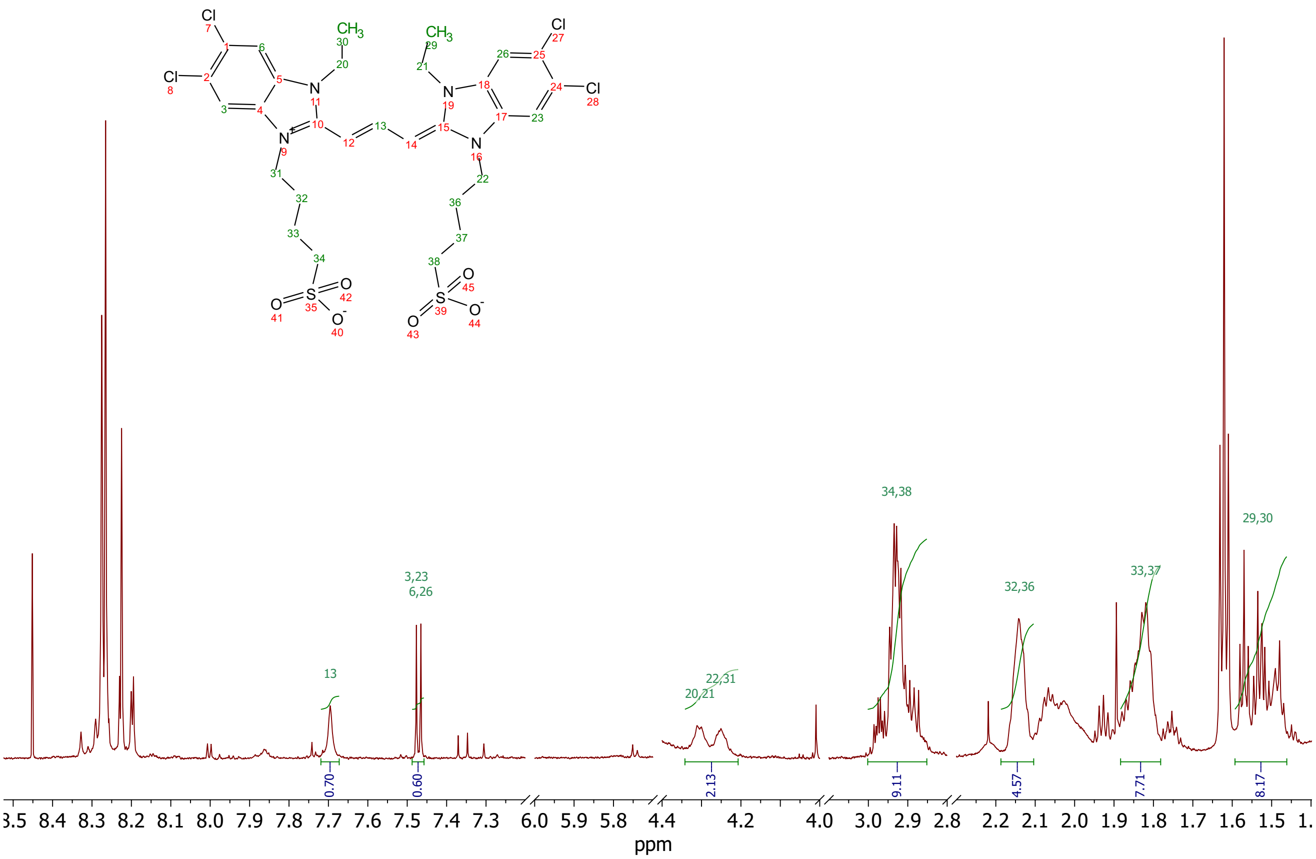

FIG. S9. ${}^1H$ NMR of TDBC in 40% MeOH

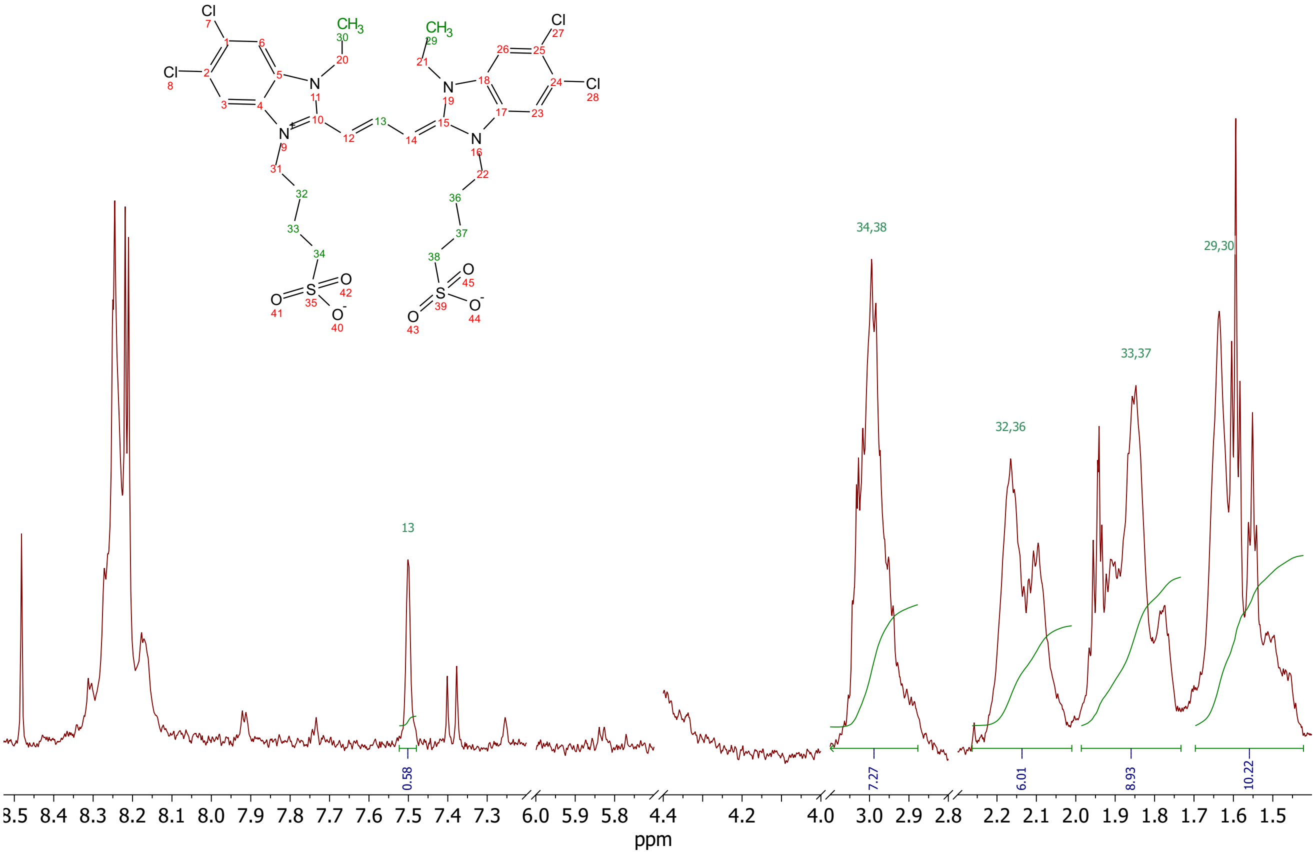


FIG. S10. $^{1}H$ NMR of TDBC in 100% $H_2O$

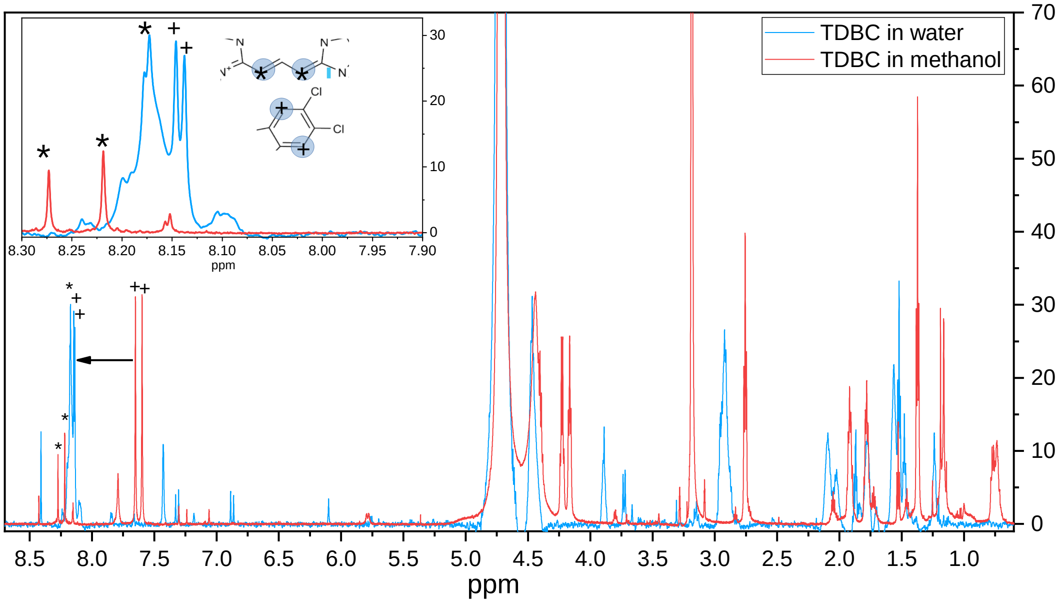


FIG. S11. 1H spectra of TDBC in methanol (red) and in water (blue). The inset shows the clustering of several resonances around $\delta$ =8.15 ppm in water due to J-aggregation.

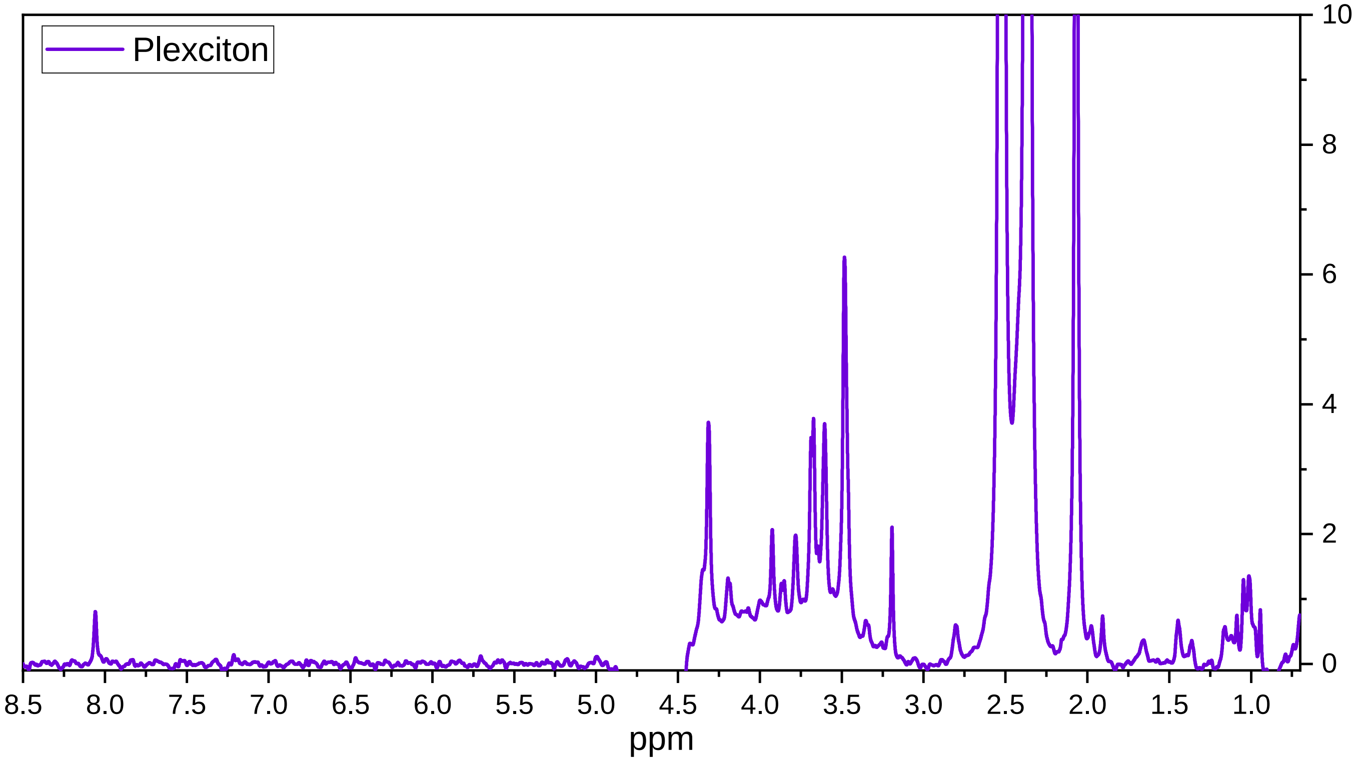


FIG. S12. 1H spectra of plexcitons in $D_2O$ using water suppression.

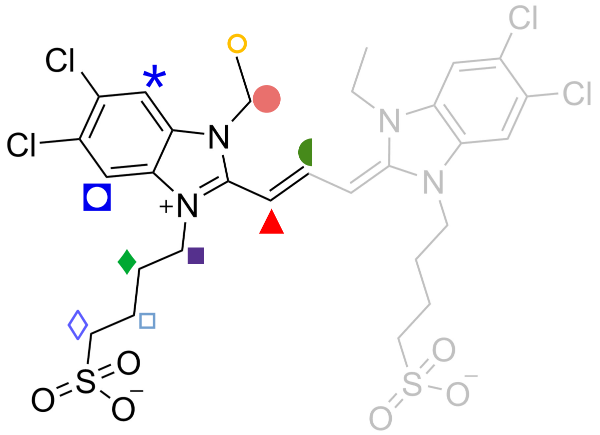


(a)

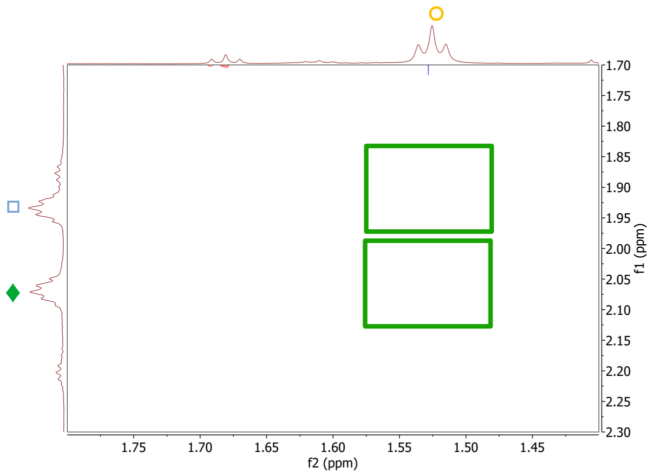


(b)

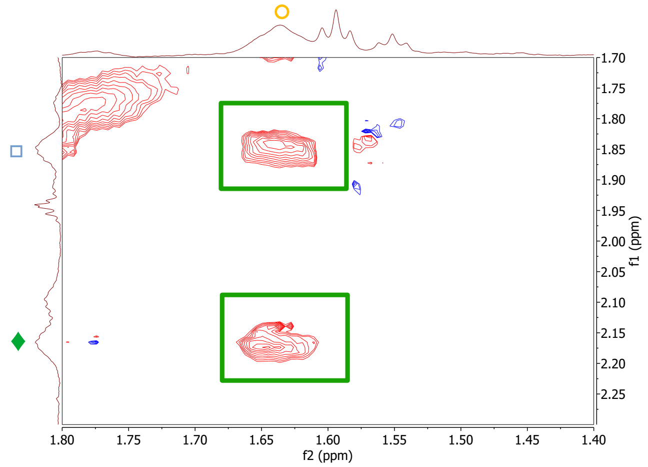


(c)

FIG. S13. NOESY spectrum of TDBC in the aliphatic–aliphatic region. (a) Molecular structure of TDBC, with one half highlighted. (b) NOESY spectrum of TDBC in methanol. The green boxes emphasize the absence of cross-peaks between spins. (c) NOESY spectrum of TDBC in water. We observe the appearance of cross-peaks which were not present in the monomeric TDBC.

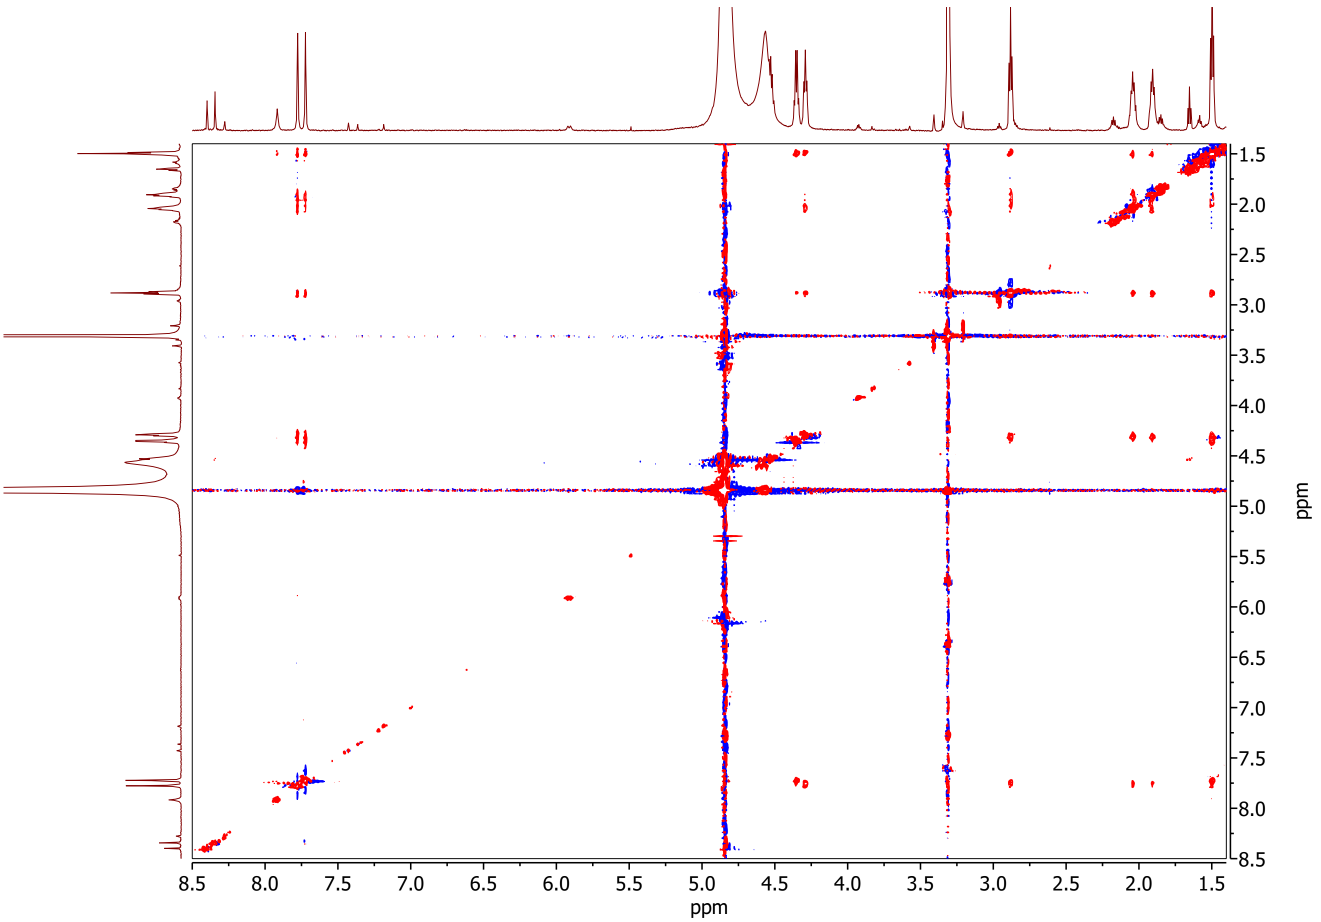


FIG. S14. NOESY spectrum of TDBC in methanol.

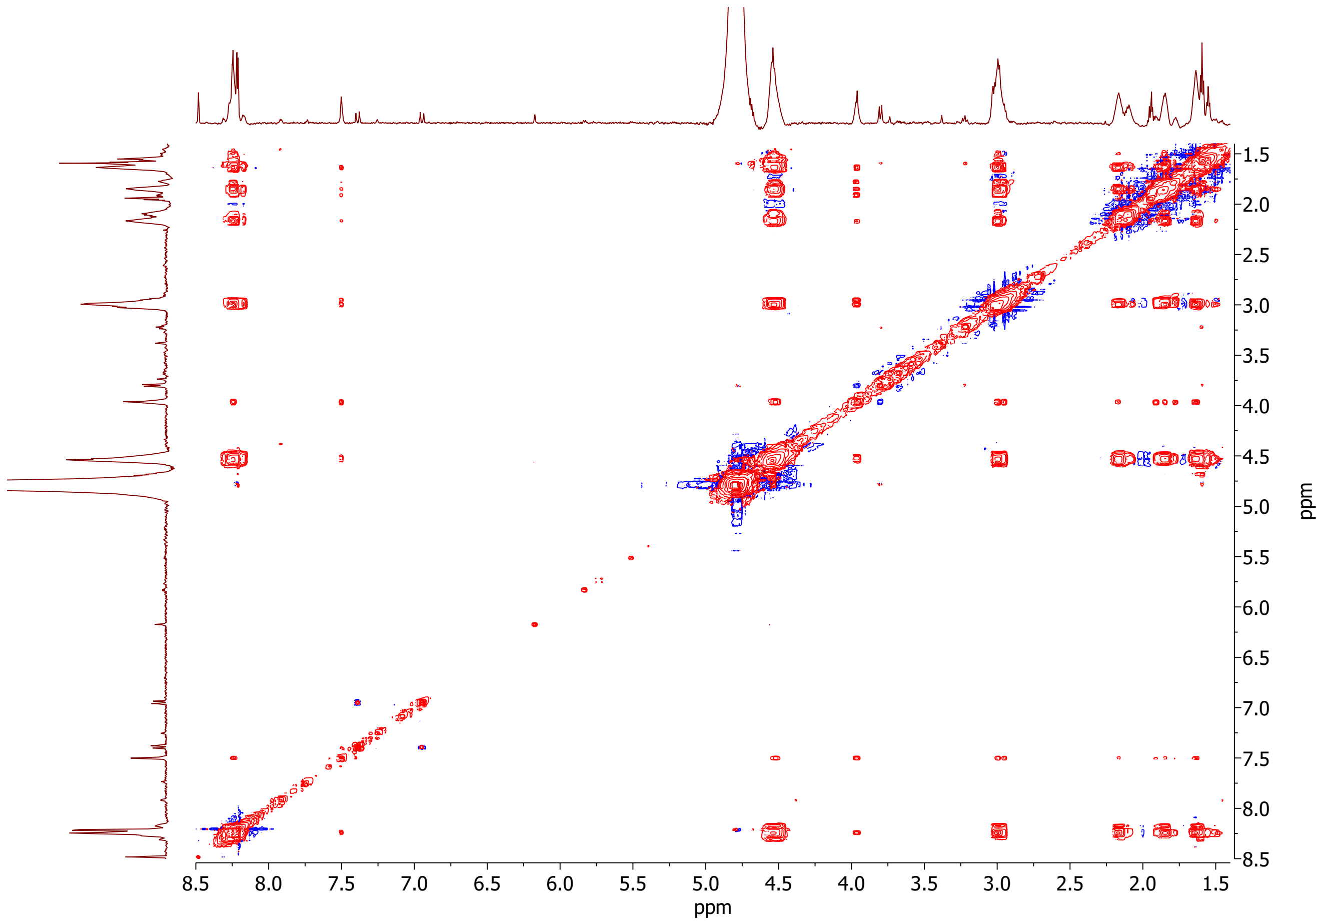


FIG. S15. NOESY spectrum of TDBC in water.

## III. RAMAN SCATTERING MEASUREMENTS

The THz-Raman without baseline correction as well as the control for pure Ag NPs is shown in Fig. S16.

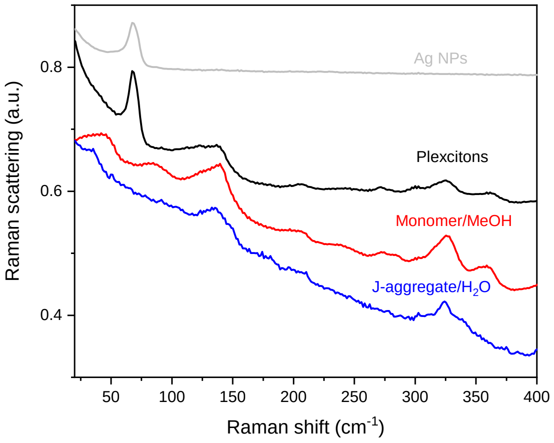


FIG. S16. THz-Raman spectra of TDBC monomer in methanol (red), TDBC J-aggregates in water (blue), plexcitons (black), and bare plasmons (purple). The 670 $cm^{-1}$ vibrational mode from the resonant Raman spectra was used as a reference for the molecular species (TDBC in methanol, TDBC in water, and the plexciton), whereas the plasmon Raman modes were referenced in amplitude to the 66 $cm^{-1}$ peak in the plexciton's THz-Raman spectrum.

## IV. VIBRATIONAL MODE ASSIGNMENT

Table S1 shows the mode assignment made from the DFT calculations. We use the H numbering shown in Fig. S17.

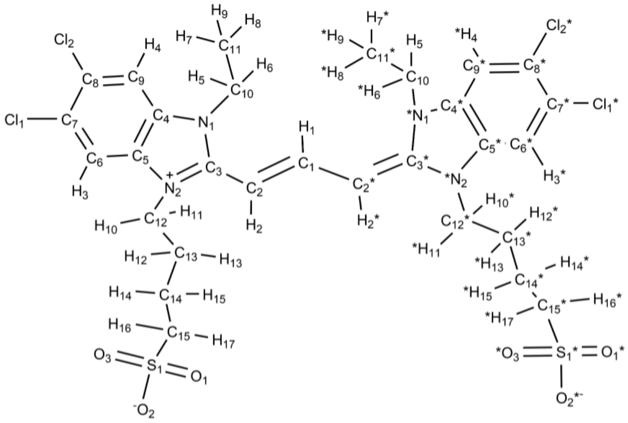


FIG. S17. TDBC structure with complete labeling of all atoms.

TABLE S1: Calculated and experimental vibrational modes of TDBC J-aggregates

| | Calculated | | Experimental | | Assignment |
|---|---|---|---|---|---|
| | opt | | | | |
| Mode | Freq (cm$^{-1}$) | Int. | Freq (cm$^{-1}$) | Int. | |
| 1 | 1632 | 0.95 | 1614 | 0.42 | In-plane motion. Deformation of benzimidazole ring and trimethine bridge. Stretching of C4-C5, C7-C8 and C2-C3. Scissoring of N1-C3-N2 and H2-C2-C1 |
| 2 | 1615 | 1.55 | 1599 | 1.02 | In-plane motion. Deformation of benzimidazole ring and trimethine bridge. Stretching of C4-C5, C7-C8 and C2-C3. Scissoring of N1-C3-N2, H2-C2-C1 and H4-C9-C8 |
| 3 | x | x | 1550 | 0.18 | xx |
| 4 | x | x | 1523 | 0.22 | xx |
| 5 | 1497 | 2.33 | 1486 | 1.57 | In-plane motion. Deformation of benzimidazole ring. Stretching of C4-C5, N1-C10. Scissoring of H4-C9-C4, H3-C6-C5, H5-C10-H6. Translation motion of hydrogen H2 and H11. |
| 6 | 1446 | 0.16 | 1453 | 0.33 | Scissoring of H10-C12-H11. Translation motion of hydrogen H2 and H3. |
| 7 | 1431 | 0.17 | 1425 | 0.25 | In-plane motion. Deformation of benzimidazole ring and trimethine bridge. Stretching of C8-C9, C6-C7,C4-C1,C5-N2. Twisting of H5-C10-H6, H10-C12-H11. Translation motion of hydrogen H2, H3 and H3. |
| 8 | 1388 | 1 | 1390 | 1 | In-plane motion. Deformation of bencene rings. Twisting of H5-C10-H6, H10-C12-H11.Wagging of Hydrogen H7,H8 , H9 and H12-C13-H13. Rocking of H3,H4 and H2 |
| 9 | 1378 | 0.24 | 1378 | 0.33 | Wagging of H12-C13-H13 and H14-C14-H15. Twisting of H10-C12-H11 and H16-C15-H17. |
| 10 | 1347 | 0.34 | x | x | In-plane motion. Deformation of bencene rings. Stretching of C4-C5, C6-C7, C7-C8 and C8-C9. Wagging of H10-C12-H11 and H14-C14-H15. Twisting of H12-C13-H13 and H5-C10-H6. Translation motion of hydrogen H2. |

*Continued on next page*

| Mode | Freq ($cm^{-1}$) | Int. | Freq ($cm^{-1}$) | Int. | Assignment |
|---|---|---|---|---|---|
| 11 | 1341 | 0.22 | x | x | In-plane motion. Deformation of benzimidazole rings. STretching of C6-C7, C8-C9 and N2-C12. Scissoring of C4-C9-H4, H3-C6-C5 and C3-C2-H2. Twisting of H10-C12-H11, H12-C13-H13, H14-C14-H15 and H5-C10-H6. |
| 12 | x | x | x | x | xx |
| 13 | 1204 | 0.45 | 1201 | 3.79 | In-plane motion. Deformation of bencene rings. Scissoring of C8-C9-H4 and H3-C6-C5. Twisting of H10-C12-H11 and H10-C12-H11. Translation motion of hydrogen H2 and H1. |
| 14 | 1159 | 0.08 | 1160 | 0.29 | Twisting of H10-C12-H11, H12-C13-H13, H14-C14-H15,H16-C15-H17 and H5-C10-H6. Stretching of S-O bond. |
| 15 | 1143 | 0.34 | 1144 | 0.26 | Twisting of hydrogens in methyl group, H5-C10-H6, H12-C13-H13, H14-C14-H15 and H16-C15-H17. |
| 16 | x | x | 1115 | 0.61 | xx |
| 17 | 1091 | 0.06 | 1087 | 0.43 | Stretching of C10-C11. Wagging of H5-C10-H6 and H7-C11-H8. Twisting of H7-C11-H9. |
| 19 | x | x | 994 | 0.22 | xx |
| 20 | 984 | 0.07 | 978 | 0.52 | In-plane motion. Deformation of bencene rings. Stretching of S1-O1, S1-O2 and S1-O3. Wagging of H4-C9-C4, H3-C6-C5, H10-C12-H11,H12-C13-H13, H16-C15-H17, H7-C11-H9 and H2-C2-C1. Twisting of H5-C10-H6 |
| 21 | 960 | 0.01 | 959 | 0.4 | In-plane motion. Deformation of bencene rings. Stretching of C7-Cl1. Wagging of H5-C10-H6 and H16-C15-H17. Twisting of H10-C12-H11, H12-C13-H13, H14-C14-H15 and H9-C11-H8 |
| 22 | 900 | 0.01 | 891 | 0.41 | Wagging of H7-C11-H9, H12-C13-H13 and H14-C14-H15. Rocking of H10-C12-H11 and H16-C15-H17. |
| 23 | x | x | 829 | 0.27 | xx |
| 24 | 807 | 0.03 | 805 | 0.34 | In-plane motion. Deformation of bencene rings. Rocking of H10-C12-H11, H16-C15-H17, H5-C10-H6 and H7-C10-H6. Translation motion of hydrogen H3, H4, H2. |
| 25 | 697 | 0.09 | 696 | 0.66 | Out-plane motion. Deformation of benzimidazole ring. Wagging of H3-midpoint of the benzene ring-H4. Twisting of C3-C2-H2. Rocking of H12-C13-H13. |
| 26 | 668.18 | 0.1 | 671 | 6.88 | In-plane motion. Deformation of benzimidazole ring. Deformation out-plane of trimethine bridge due Twisting of H2. Rocking of H10-C12-H11, H14-C14-H15. |
| 27 | x | x | 655 | 0.28 | xx |
| 28 | x | x | 642 | 0.51 | xx |
| 29 | x | x | 633 | 1.05 | xx |
| 30 | x | x | 617 | 0.61 | xx |
| 31 | x | x | 585 | 0.34 | xx |
| 32 | x | x | 557 | 0.55 | xx |
| 33 | x | x | 527 | 0.63 | xx |
| 34 | 509 | 0.02 | 500 | 0.51 | In-plane motion. Rocking of H3-midpoint of the benzene ring-H2 and the entire butane chain. |
| 35 | 469 | 0.01 | 470 | 1.77 | Out-plane motion. Deformation of benzimidazole ring trimethine bridge. Translaton motion of H3, H4, N1,C3 and H2.Rocking of H10-C12-H11. Wagging of H5-C10-H6 |
| 36 | 439 | 0.02 | 446 | 0.88 | Out-plane motion. Deformation of bencene rings . Rocking of H5-C10-H6. Wagging of H3-midpoint of the benzene ring-H2. Translation motion of hydrogen H2 in-plane. |
